# Supplementary material for: MultiSPANS: A Multi-range Spatial-Temporal Transformer Network for Traffic Forecast via Structural Entropy Optimization
Source: arXiv:2311.02880 source file (2023-11-06)
Supplement: Supplementary file 1 [file Appendix.tex]

%\clearpage
%\section{METHODS}\label{sec:appendix1}
